# Supplementary material for: Interactive Code Generation via Test-Driven User-Intent Formalization
Source: arXiv:2208.05950 source file (2023-10-04)
Supplement: Supplementary file 1 [file appendix.tex]

\appendix

\section{Caveats of Evaluating User Interaction}
\label{sec:threats}

Although the problem formulation above allows us to evaluate the quality of the solutions in a completely automated manner, we note some subtleties due to the use of an incomplete hidden test-suite and the use of the reference solution.  

First, we inherit the  well known {\it false positive} issue in program synthesis related to the incompleteness of test suites as the correctness specification for code~\cite{alphacode_2022}.
It admits degenerate solutions $f'$ that only satisfy the exact input output pairs in the unit tests in $T_p$, but do not generalize to satisfy the intent of the user for most other inputs. 

Second, the incompleteness of hidden tests also leads to unexpected situations where pruning incorrect code using user feedback can reduce the pass@1.
Consider the case where the user wants to generate code satisfying the natural language description 
\begin{lstlisting}[style=mystyle]
def double(x):
    """double an integer"""
\end{lstlisting}
Let us also assume that the reference implementation consists of 
\begin{lstlisting}[style=mystyle]
def double(x):
    """double an integer"""
    return x + x
\end{lstlisting}
The unit test suite $T_p$ consists of a single test $(2, 4)$.

Let us assume that a model generates a code suggestion:
\begin{lstlisting}[style=mystyle]
def double(x):
    """double an integer"""
    return 4
\end{lstlisting}

The pass@1 metric for this set of suggestions (without any interaction) is 1, since the code suggestion satisfies the hidden tests.
Consider the case when the user is presented with a generated test $(1, 2)$.
Since this test is consistent with user intent (and satisfied by the reference solution), a user would respond \yesResponse.
This results in pruning the solution returning $4$, resulting in pass@1@1 to be 0, lower than pass@1. 
\shuvendu{Iterate that this does not have anything to do with using the reference solution.}

Finally, the idea of using the reference solution to determine user response may (in rare cases) not capture the cognitive cost on a user inspecting the presented test. 
Consider the case when a test $(i, o)$ satisfies the reference solution $f_p$, and we therefore simulate the user response as \yesResponse.
However, for the case when the test presents a query that is difficult for the user to determine --- say,  $\texttt{IsFib}(99545) == \texttt{True}$! 
A user may say \dnResponse{} for such a query to ignore such a test, even though it can be evaluated to a definite value by the reference (correct) implementation of $\texttt{IsFib}$.
